# Supplementary material for: Diffusion-Aided Joint Source Channel Coding For High Realism Wireless Image Transmission
Source: arXiv:2404.17736 source file (2025-03-22)
Supplement: Supplementary file 1 [file appendix.tex]

\appendices
\section{\textcolor{blue}{Ablation Studies on $\lambda_c$ and $\lambda_g$}}

\textcolor{blue}{An ablation study of $\lambda_c$ and $\lambda_g$ was conducted on CIFAR-10 to better illustrate their effect. For the ablation study of $\lambda_c$, we set $\lambda_g=0, N_s=6, N_p=1$ and $SNR=5dB$. The results of PSNR and channel estimation MSE are shown in Table. \ref{tablambdac}. Obtained PSNR is not sensitive to $\lambda_c$ although setting $\lambda_c = 0$ results in significantly larger channel estimation error. Using channel estimation subnet $\Phi_{ce}$ enhances the quality of the image as shown in Table \ref{tab1} and \ref{tab2}. Although the image quality does not significantly depend on $\lambda_c$, applying $\lambda_c > 0$ produces more interpretable trained results from the channel estimation subnet.}

\textcolor{blue}{For the ablation study of $\lambda_g$, we set $\lambda_c=0.5, N_s=6, N_p=1$ and $SNR=5dB$. As we gradually increase $\lambda_g$, the reconstruction PSNR drops while the classification accuracy increases. When $\lambda_g$ gets too large, however, the neural network tends to create (fake) contents that are differ from original images, degrading both PSNR and classification accuracy. To visualize it, we show examples from CIFAR-10 in Figure \ref{fig:fig_visual_lambdag}. }
\tableabc
\tableabg
\figvisuallambda
% you can choose not to have a title for an appendix
% if you want by leaving the argument blank

\section{\textcolor{blue}{Comparison with other JSCC structures}}
\textcolor{blue}{We compare our basic neural network structure without OFDM and subnets (i.e., 'Direct w/o OFDM') with those proposed in \cite{bourtsoulatze2019deep} and \cite{burth2020joint}. We conduct experiments on CIFAR-10 using AWGN and multipath fading channels. As we exclude OFDM from our scheme, the difference only comes from the neural network structure itself. For each 32 $\times$ 32 image, we assign 384 channel usages, yielding a CPP of 0.375. The evaluation results are shown in Figure \ref{fig:fig_net_result}. Our structure constantly outperforms the other structures in both AWGN channel and multipath fading channels whereas our structure uses 23\% fewer parameters than the structure in \cite{burth2020joint}. Our performance further improves in the multipath fading channel as we incorporate OFDM blocks as well as proposed subnet structures (`OFDM+CE+EQ+$\Phi_{ce}$+$\Phi_{eq}$').}
\fignetresult
